# Supplementary material for: Physics-aware Spatiotemporal Modules with Auxiliary Tasks for Meta-Learning
Source: arXiv:2006.08831 source file (2021-06-07)
Supplement: Supplementary file 1 [file appendix.tex]

\section{Task 1: Multi-step Graph Signal Generation}
\subsection{Meta-train}
\label{ap:meta-train}
\textbf{Data}: For all experiments, we generate the data for meta-train tasks from a sum of sinusoidal functions with different spatial frequencies (Eq.~\ref{eq:synthetic-ap}). 

\begin{equation}
\begin{aligned}
    u(x,y) =\sum_{|k|,|l| \leq F} \lambda_{k, l}& \cos (k x+l y)+\gamma_{k, l} \sin (k x+l y),\\&\text{where }~\lambda_{k,l},\gamma_{k,l}\sim\mathcal{N}\left(0,0.02\right),
\end{aligned}
\label{eq:synthetic-ap}
\end{equation}
where $(x,y)$ in the 2D space $([0,2\pi]\times[0,2\pi])$ and $k, l$ are randomly sampled integers. 
Once the spatially continuous function values are generated, we uniformly sample different number of locations from all grid points as observed nodes to simulate the case where the observations are irregularly distributed in space. 
We then construct a $k$-Nearest Neighbor graph based on the Euclidean distance as the input of graph neural networks.
The combination of parameters to generate the synthetic dataset is given in Table~\ref{tab:syn-data-ap}.
We construct 100 snapshots per a combination of the parameters $(N,E,F)$ using a unique random seed. 
75 snapshots per each combination are used for $\gD^{tr}$ and 25 snapshots are for $\gD^{te}$.

\begin{table}[h]
% \vspace{-1em}
\centering
\small
\begin{tabular}{@{}ccc@{}}
\toprule
& Meta-train & Meta-test \\ \midrule
\# nodes ($N$) & \{256, 625\} & \{450, 800\} \\
\# edges per a node ($E$) & \{4, 8\} & \{3, 6, 10\}      \\
Initial frequency ($F$) & \{2, 5\} & \{3, 7\} \\ \bottomrule
\end{tabular}
\caption{Parameters for synthetic dataset}
\label{tab:syn-data-ap}
\end{table}

\textbf{Tasks}: For each node, we have the first and second order derivatives.
We meta-train the spatial derivative modules (Sec. 3.1) to predict the spatial derivatives by feeding node and edge features (function value at a node and relative displacement, respectively) as input.

% Each sequence lasts 20 frames with the timestep size 0.01. We set up 1 $k$-shot meta-train task on each sequence: predicting the values and 1st/2nd-order spatial derivatives on all nodes for all frames with an auto-regressive model given the first frame as the input. The first $k$ frames are used for training and the rest $20-k$ frames for test. We select $k=5,10$ as two experiment settings.

% \begin{figure}[h]
%     \centering
%     \includegraphics[width=\textwidth,height=3cm]{example-image-a}
%     \caption{Visualization of the synthetic data and spatial gradients.}
%     \label{fig:synthetic-dynamics-gradients}
% \end{figure}

\subsection{Meta-test}
\subsubsection{Synthetic}
% \begin{itemize}
%     \item Visualization of dynamics
%     \item Visualization of first-order gradients (arrows?)
%     \item Visualization of second-order gradients (arrows?)
% \end{itemize}
\textbf{Data}: We generate the synthetic meta-test data from Eq.~\ref{eq:synthetic-ap} but set different parameters to simulate the realistic scenario where meta-train tasks and meta-test tasks do not share the same distribution.

\textbf{Tasks}: We reuse the spatial modules in \ref{ap:meta-train} to evaluate how the meta-initialized parameters are easily adaptable to unseen graph signals with different spatial resolution, discretization, and the degree of function fluctuation. 
We use 15 snapshots for the adaptation in meta-test and 75 snapshots are used to evaluate the proposed model.

\subsubsection{Real-world Dataset} \label{ap:real-world-single}

\textbf{Data}:

\textbf{AQI-CO}~\cite{aqi2017}: There are multiple pollutants in the dataset and we choose carbon monoxide (CO) ppm as a target pollutant in this paper.
We select sensors located in between latitude (26, 33) and longitude (115,125) (East region of China).
In this region, we sample multiple multivariate time series whose length should be larger than 12 steps (12 hours) for multiple meta-tasks.
There are around 60 working sensors and the exact number of the working sensors is varying over different tasks.
Fig.~\ref{fig:sensors} shows the locations of selected AQI sensors.
    
\textbf{ExtremeWeather}: We select the data in the year 1984 from the extreme weather dataset in \cite{racah2017extremeweather}. The data is an array of shape (1460, 16, 768, 1152), containing 1460 frames (4 per day, 365 days in the year). 16 channels in each frame correspond to 16 spatiotemporal variables. Each channel has a size of 768$\times$1152 corresponding to one measurement per 25 square km on earth. For each frame, the dataset provides fewer than or equal to 15 bounding boxes, each of which labels the region affected by an extreme weather event and one of the four types of the extreme weather: (1) tropical depression, (2) tropical cyclone, (3) extratropical cyclone, (4) atmospheric river. In the single feature setting, we only utilize the channel of surface temperature (TS).% We focus on events of the type (2) tropical cyclone for all experiments.

\begin{figure}[t]
    \centering
    \includegraphics[width=0.4\linewidth]{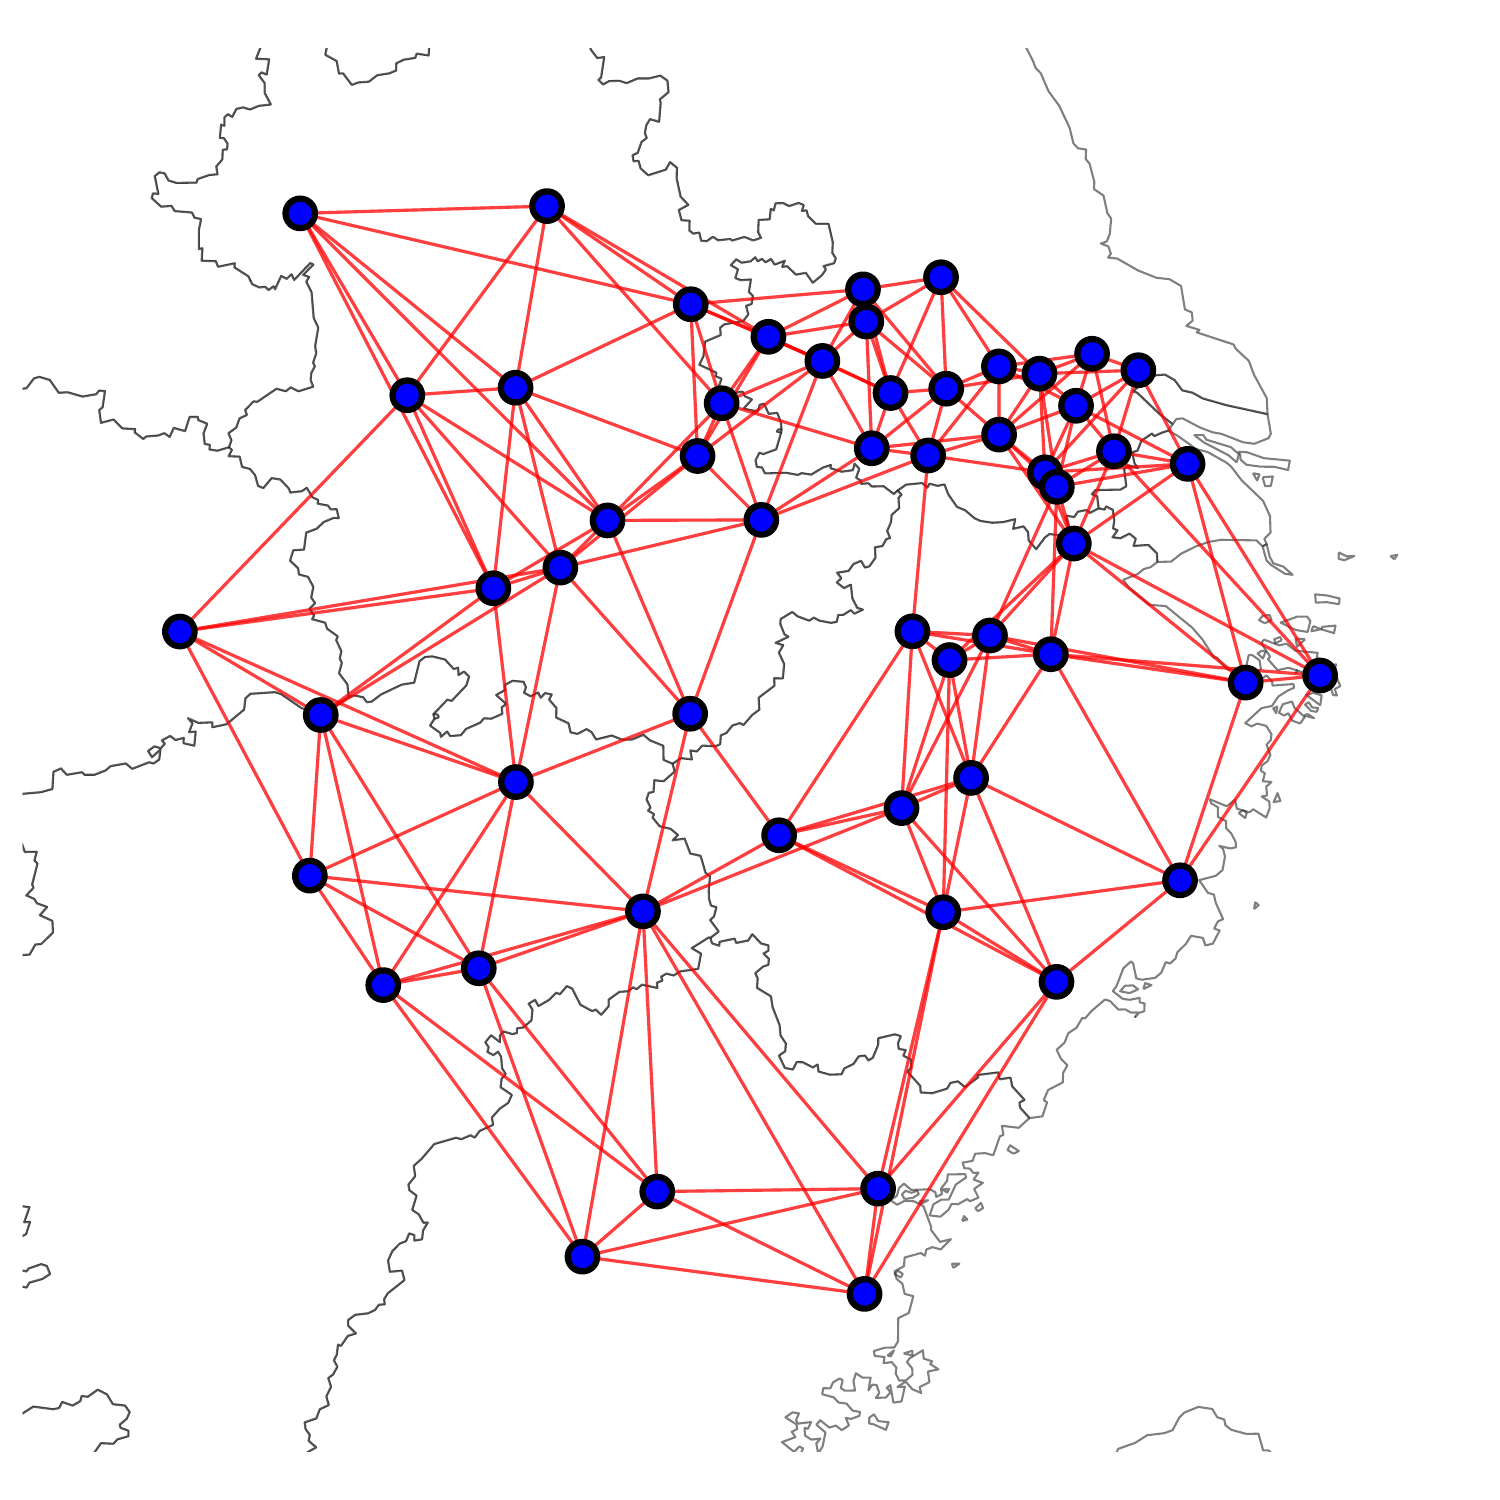}
    \caption{Sensor locations in the AQI-CO dataset. 
    We show sensors as blue nodes and edges of $k$-NN graphs as red lines. Borders of provinces are shown in grey.}
    \label{fig:sensors}
\vspace{-2em}
\end{figure}

\textbf{Tasks}:

\textbf{AQI-CO}: We select the first sequence of carbon monoxide (CO) ppm records from each month in the year 2015 at land-based stations, and set up the meta-test task on each sequence as the prediction of CO ppm. We construct a 6-NN graph based on the geodesic distances among stations.

\textbf{ExtremeWeather}: First, we aggregate all bounding boxes into multiple sequences. In each sequence, all bounding boxes (1) are in consecutive time steps, (2) are affected by the same type of extreme weather, and (3) have an intersection over union (IoU) ratio above 0.25 with the first bounding box in the sequence. Then we select the top-10 longest sequences. For each sequence, we consider its first bounding box $A$ as the region affected by an extreme weather event, and extend it to a new sequence of 20 frames by cropping and appending the same region $A$ from successive frames. For each region we uniformly sample 10\% of available pixels as observed nodes to simulate irregularly spaced weather stations and build a 4-NN graph based on the Euclidean distance. Fig.~\ref{fig:extremeweather} visualizes the first 5 frames of one extended sequence. In the single feature experiment, we set up a meta-test task on each extended sequence as the prediction of the surface temperature (TS) on all observed nodes with the initial TS given only.

\subsection{Experimental Details}

\begin{figure*}[t]
    \centering
    \includegraphics[width=\linewidth]{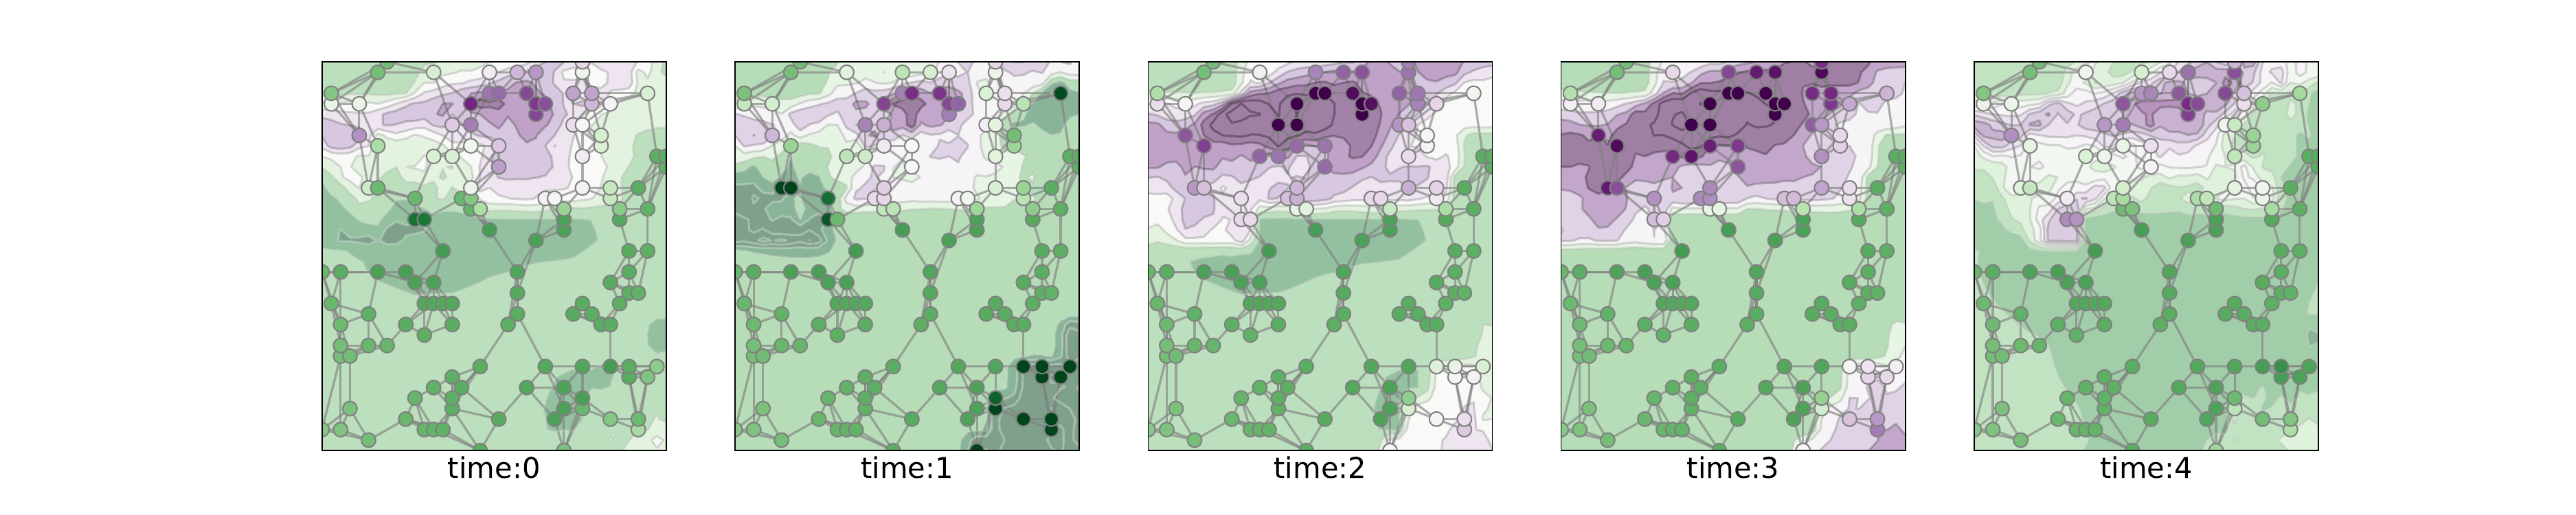}
    \caption{Visualization of the first 5 frames of one extended sequence in the extreme weather dataset. Dots represent the sampled points. Greenish (purplish) area is higher (lower) surface temperature.}
    \label{fig:extremeweather}
\end{figure*}

\begin{figure*}[t]
    \centering
    \subfigure{\includegraphics[width=0.23\linewidth]{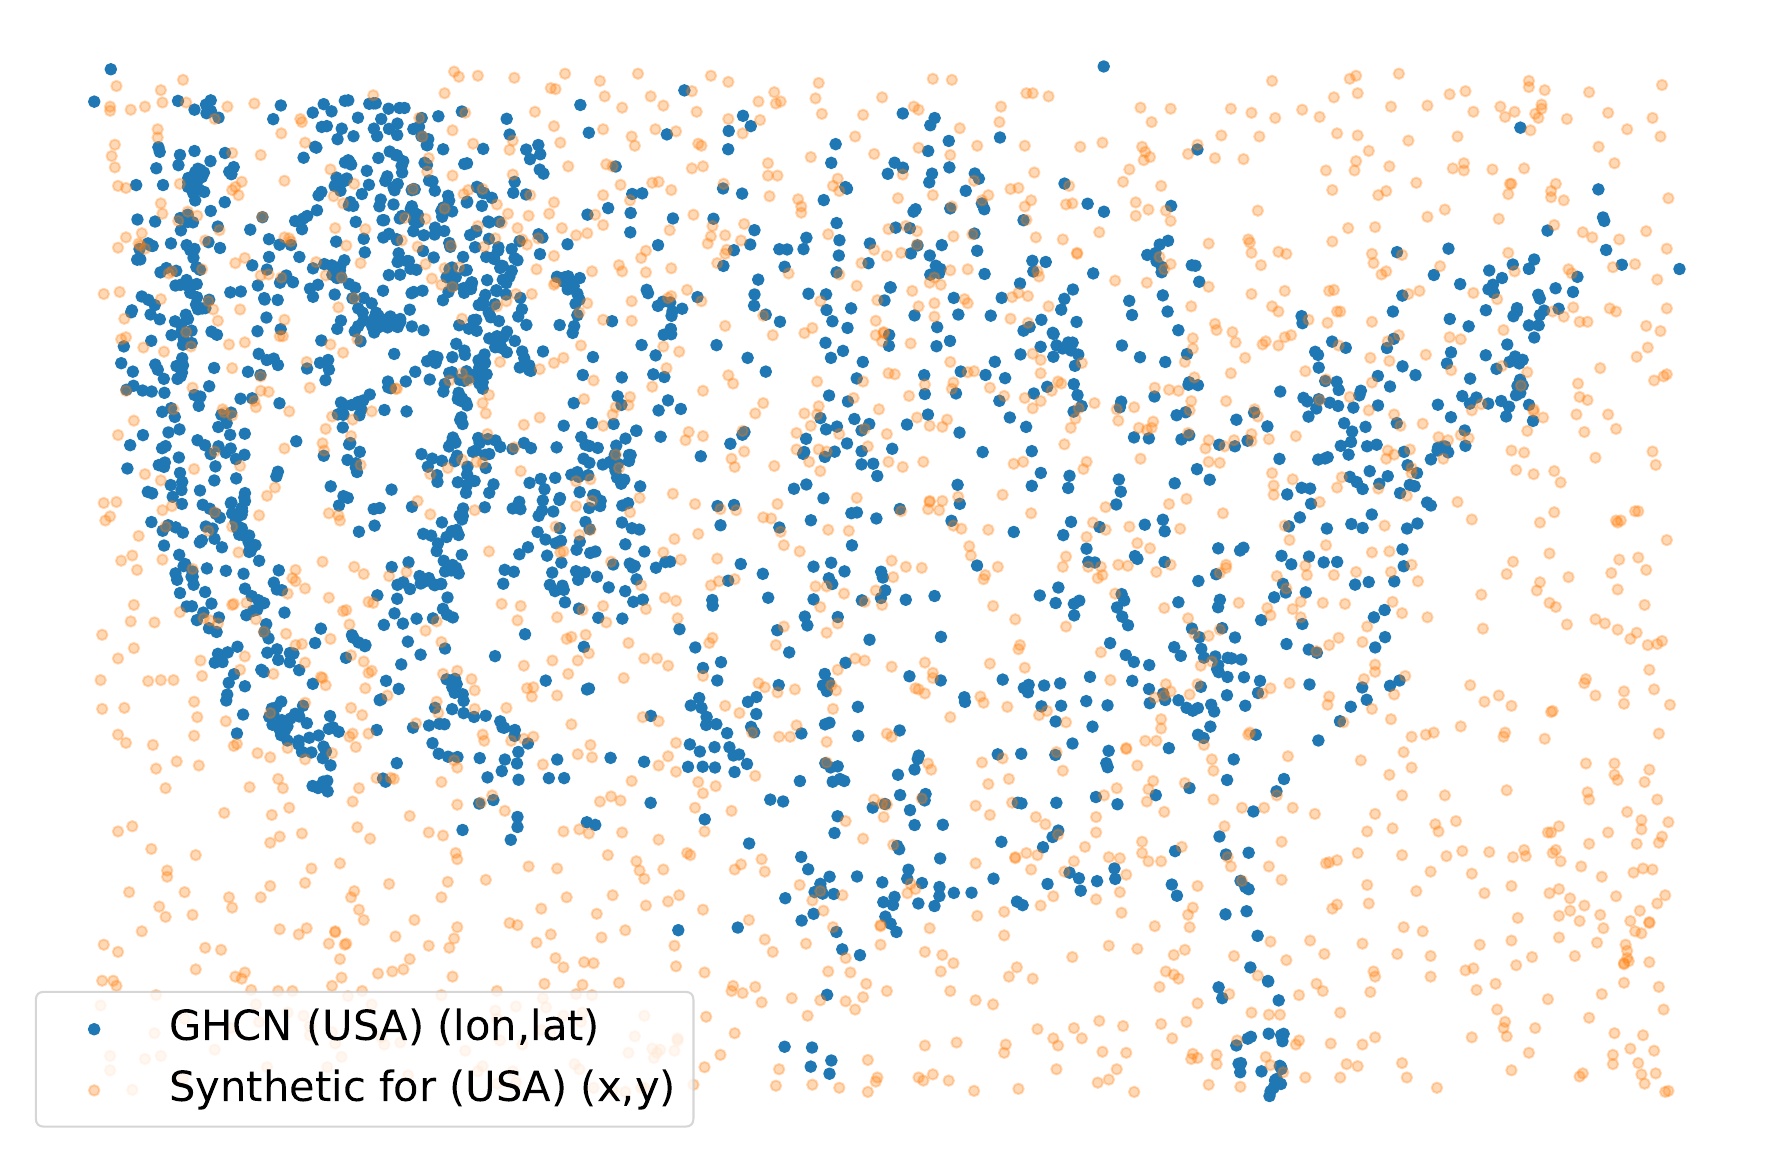}}
    \hfill
    \subfigure{\includegraphics[width=0.23\linewidth]{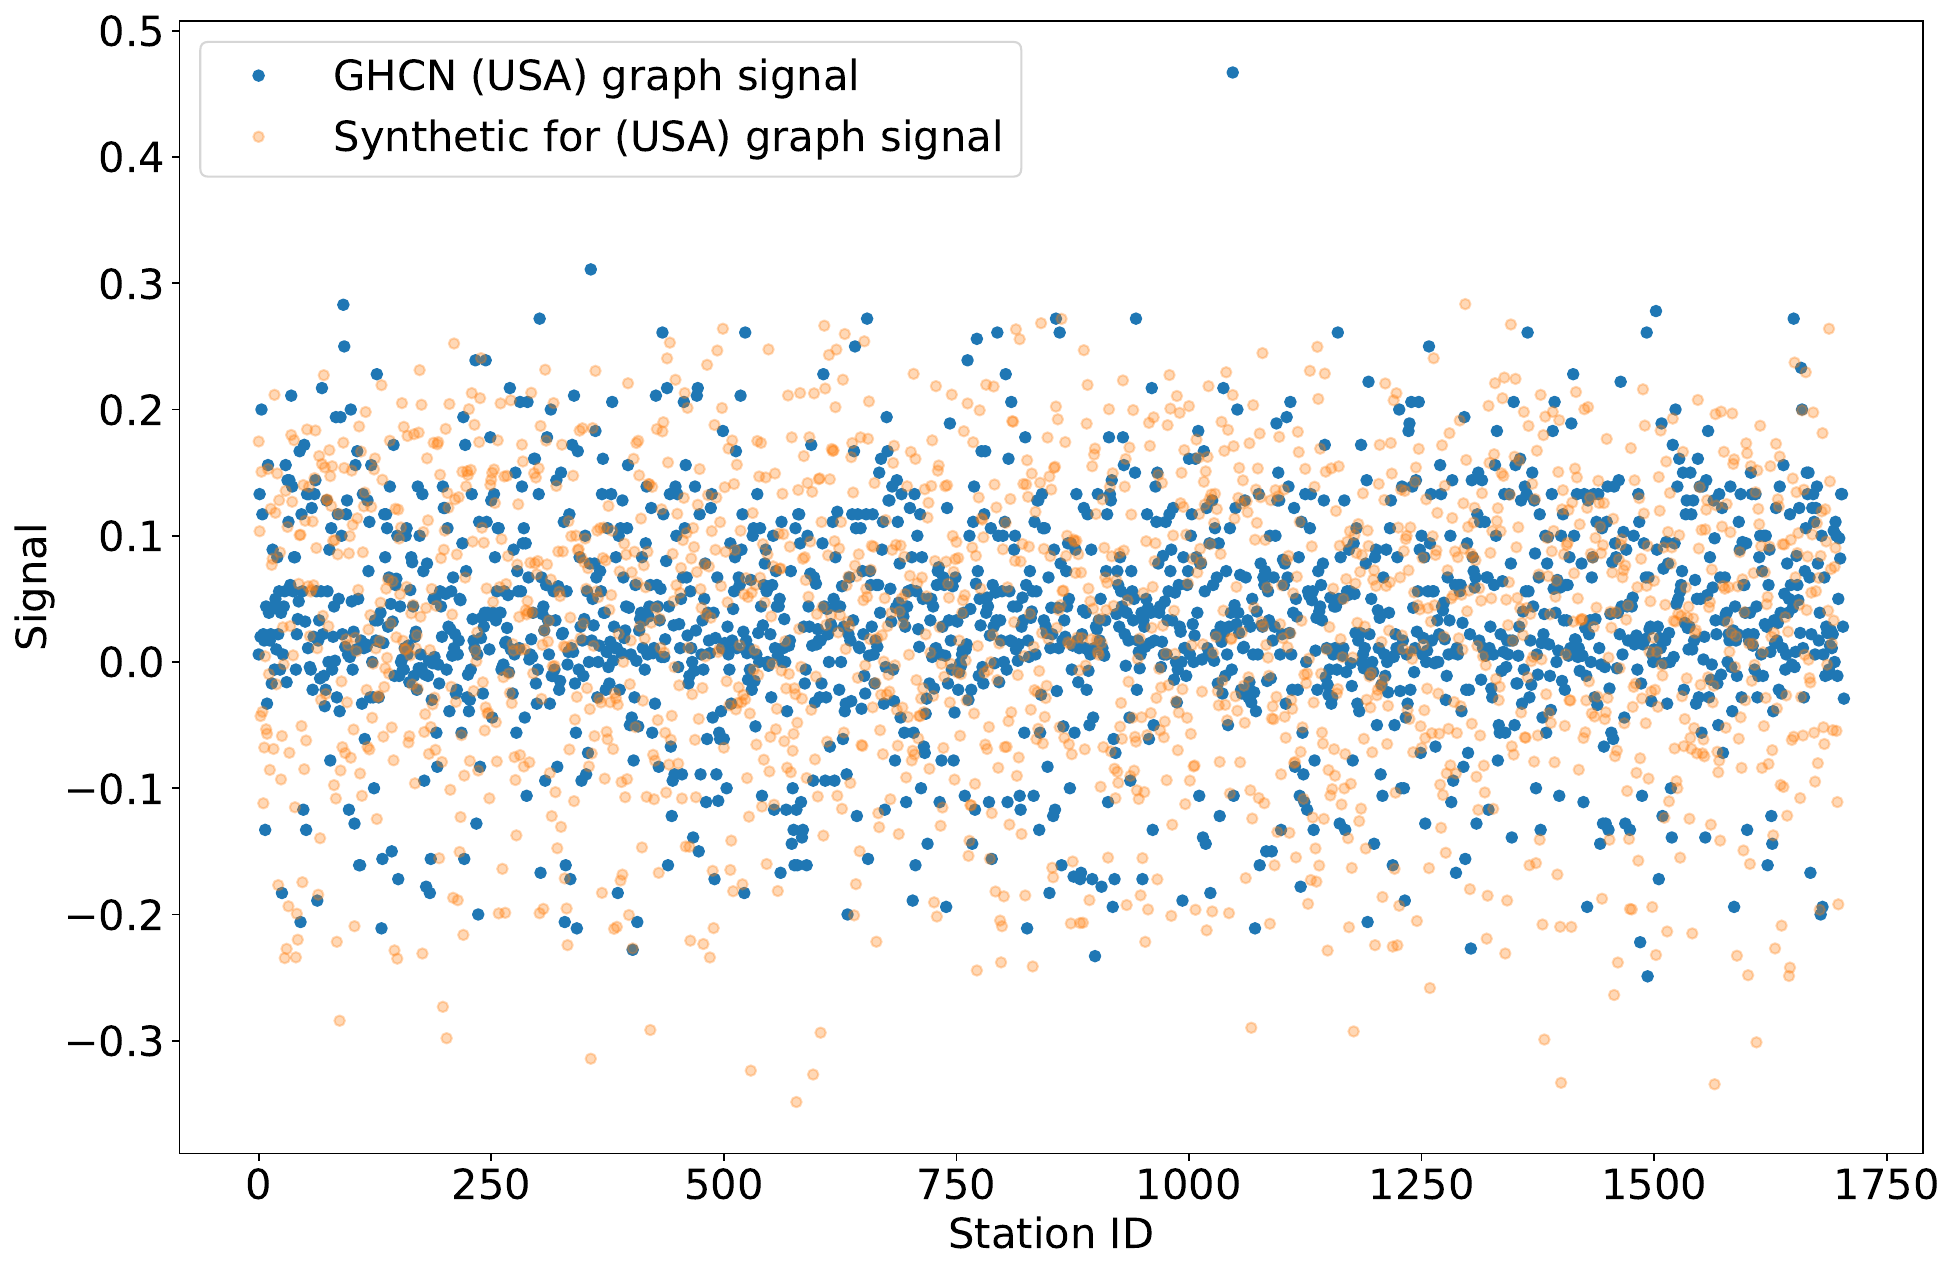}}
    \hfill
    \subfigure{\includegraphics[width=0.23\linewidth]{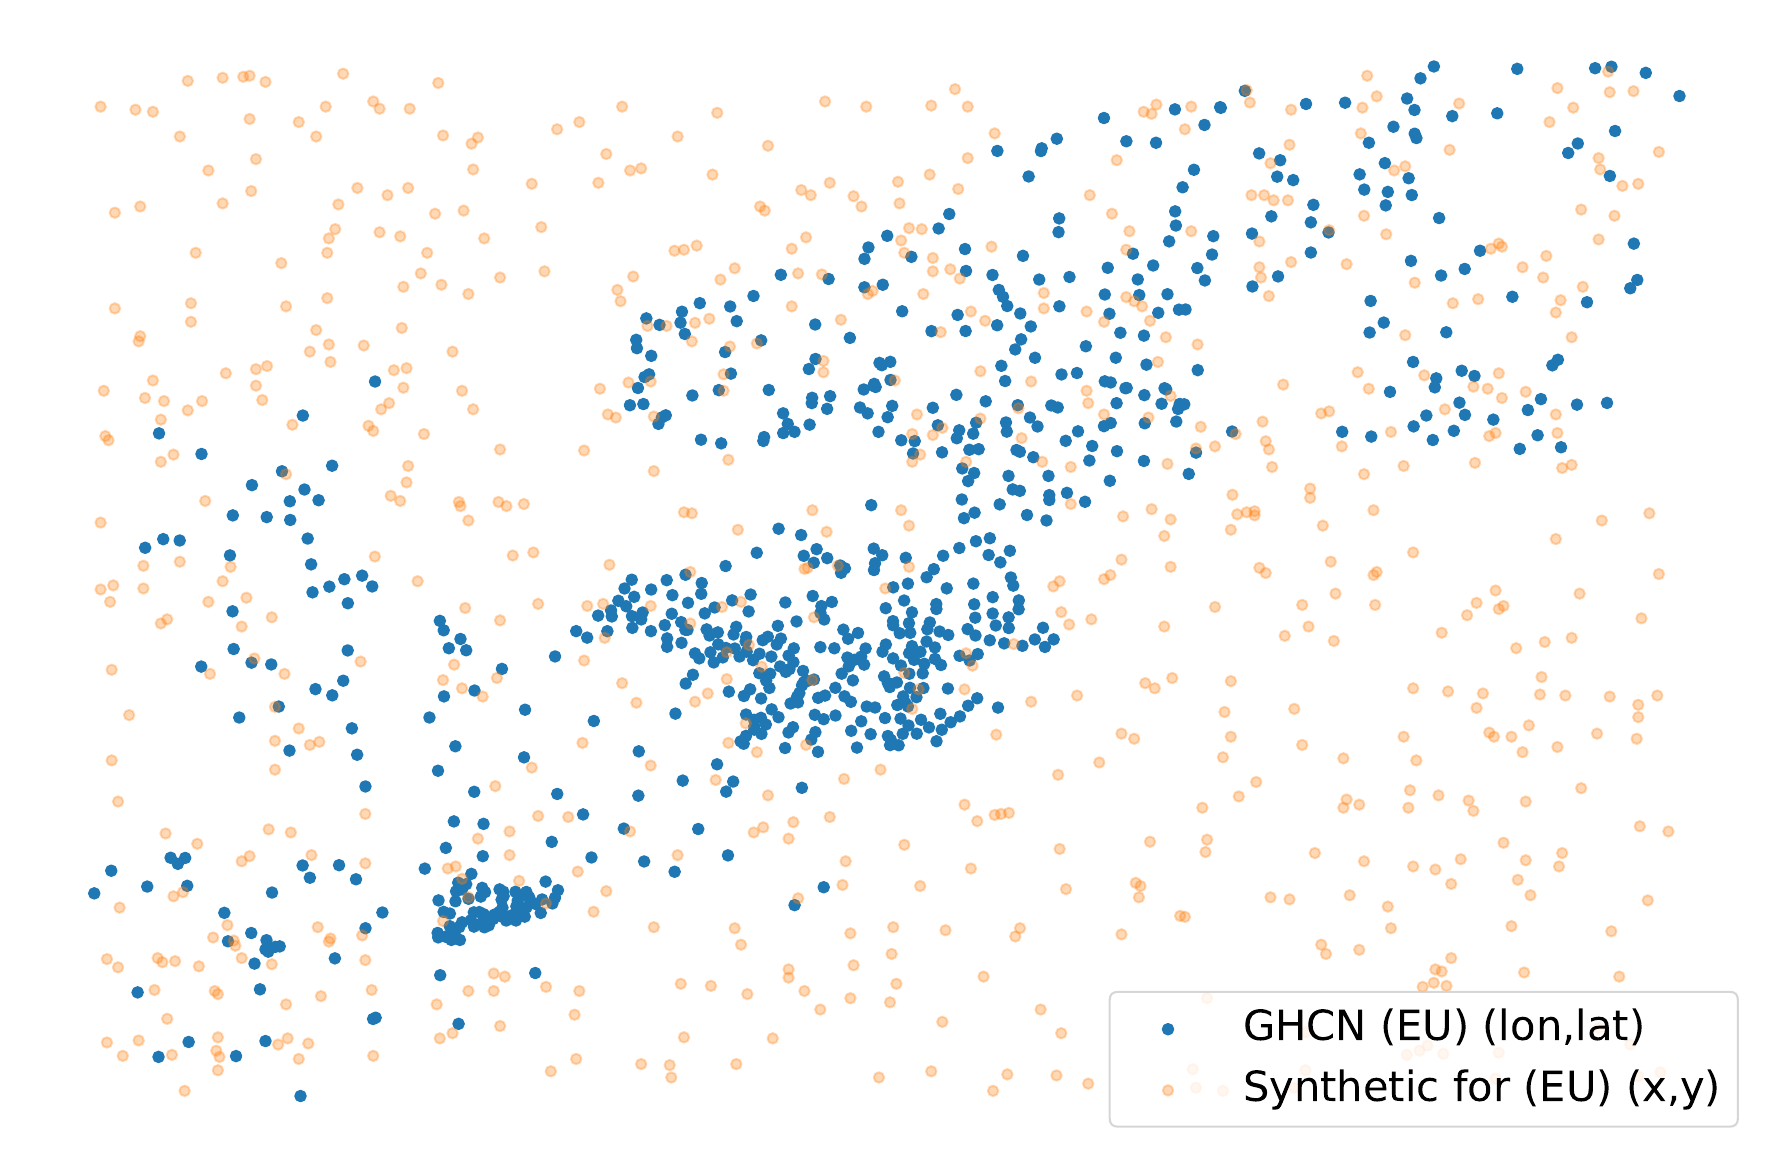}}
    \hfill
    \subfigure{\includegraphics[width=0.23\linewidth]{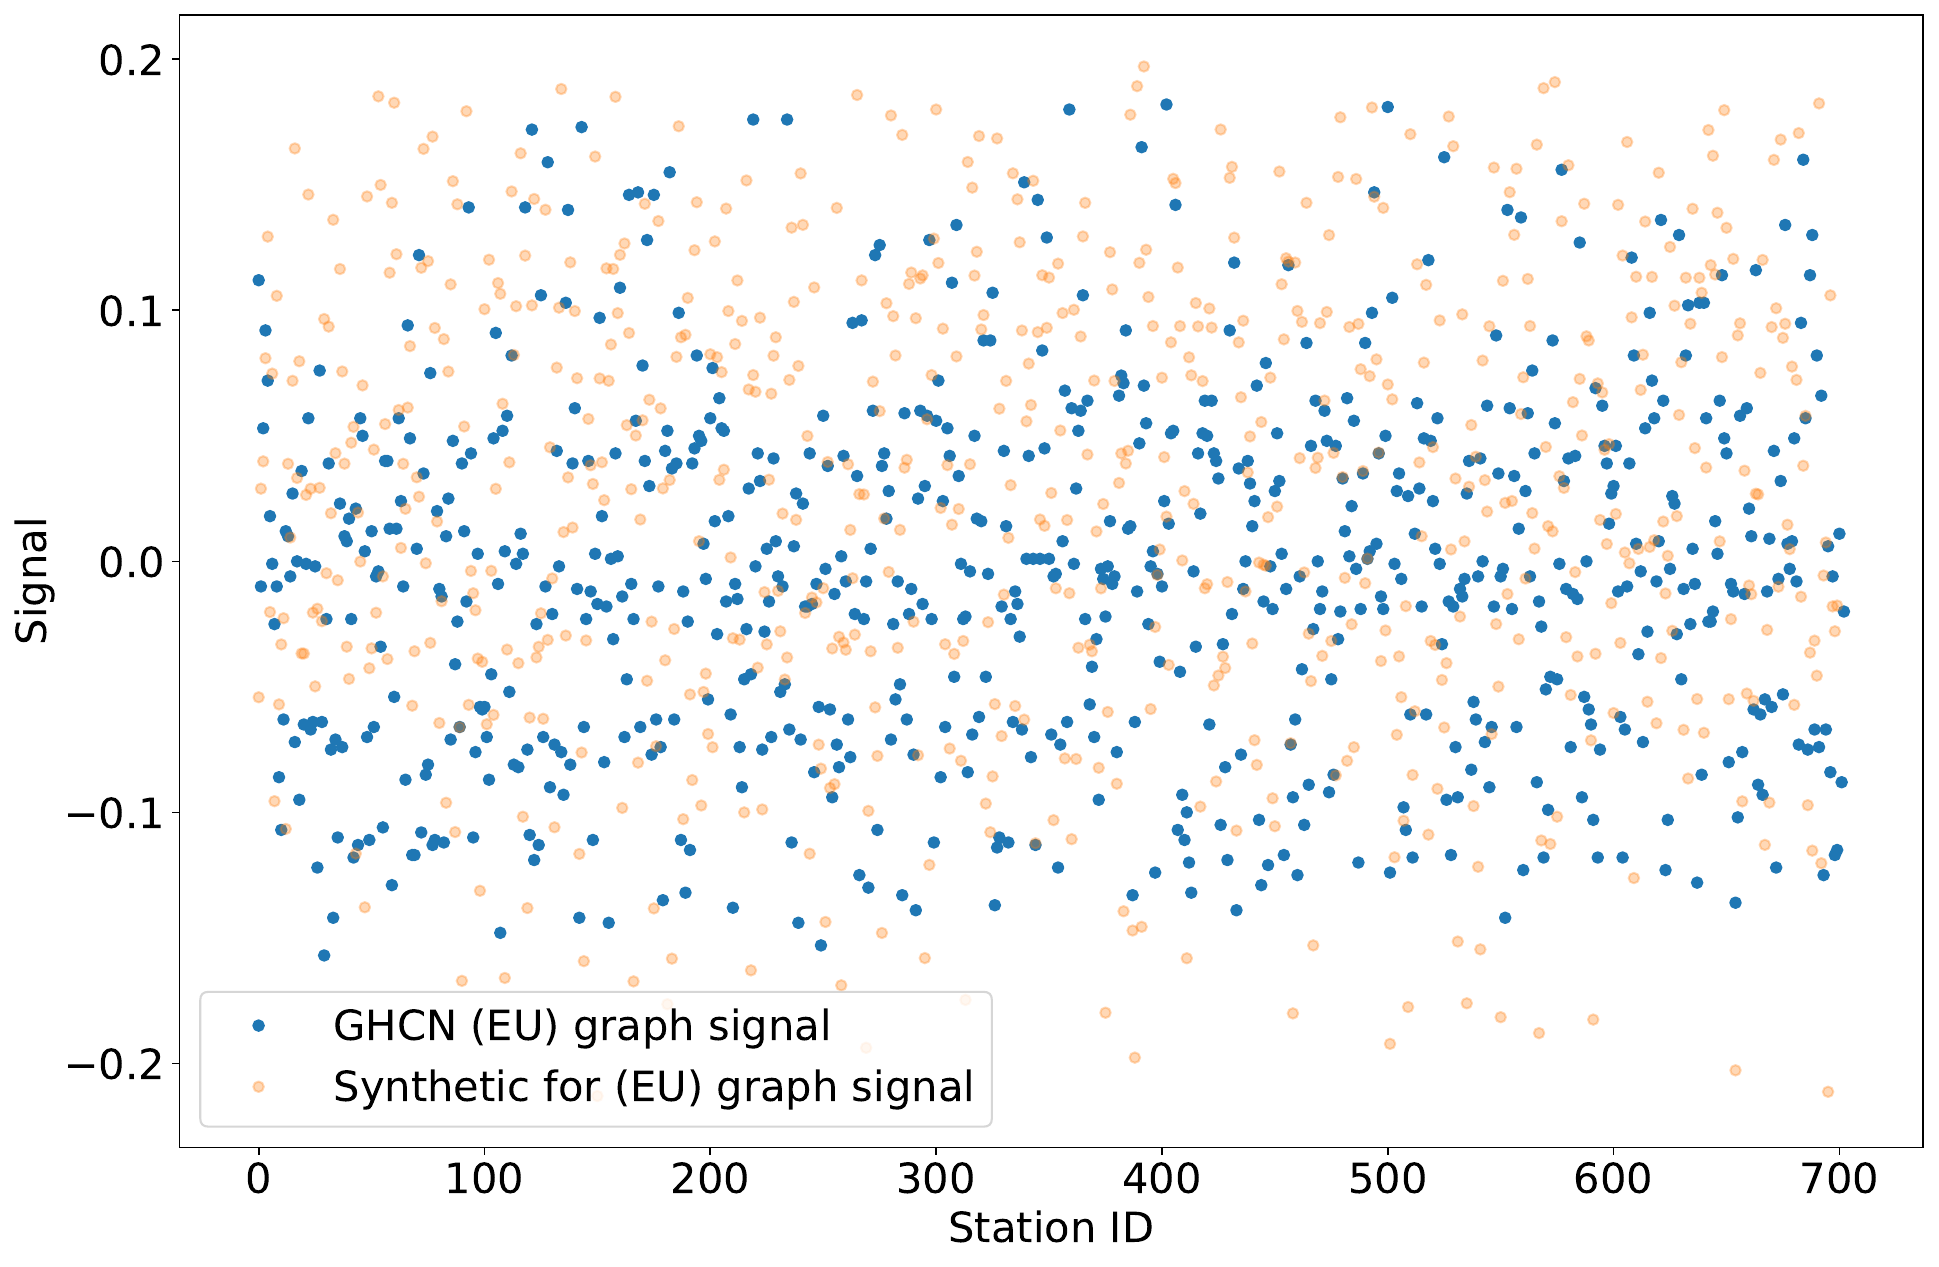}}
    \caption{(first and third) Spatial distribution of the GHCN weather stations and synthetic nodes. (second and fourth) Function values of the GHCN records and synthetic function.}
    \label{fig:append-ghcn-syn}
    % \vspace{-4mm}
\end{figure*}

\subsubsection{Baselines}

\textbf{PA-DGN (train from scratch)}~\cite{Seo*2020Physics-aware}: For each meta-test task, initialize one PA-DGN model randomly and train it on the single task.
The spatial derivative layer uses a message passing neural network (MPNN) with 2 GN blocks using 2-layer MLPs as update functions. The forward network part uses a recurrent graph  neural network with 2 recurrent GN blocks using 2-layer GRU cells as update functions. We set its hidden dimension to 64, in which case PA-DGN has a similar number of parameters with RGN. The PA-DGN model has 384,653 learnable parameters.

\subsubsection{Ours}

\textbf{PiMetaL}: Meta-train the spatial derivative modules (SDM) with our proposed Alg. 3 on the meta-train tasks generated in~\ref{ap:meta-train}.
Then for each meta-test task, initialize one time derivative module (TDM) randomly and output of SDM is fed into the TDM to train it on the single task.
The architecture for SDM and TDM are identical for the spatial derivative layer and the recurrent graph network in PA-DGN, respectively.

\subsubsection{Training Settings}
\textbf{Training hyperparameters}: For all meta-train and meta-test tasks, we use the Adam optimizer with the learning rate 1e-3. In each training epoch, we sample 1 task from all available tasks.

\textbf{Environments}: All experiments are implemented with Python3.6 and PyTorch 1.3.0, and are conducted with NVIDIA GTX 1080 Ti GPUs.

\textbf{Runtime}: The baselines RGN (train from scratch) and PA-DGN (train from scratch) will finish in 30 minutes. All other baselines will finish the meta-train stage in 4 hours and the meta-test stage in 2 hours. The runtime is measured in environments described above.

\begin{figure}[t]
    \centering
    \subfigure{\includegraphics[width=0.45\linewidth]{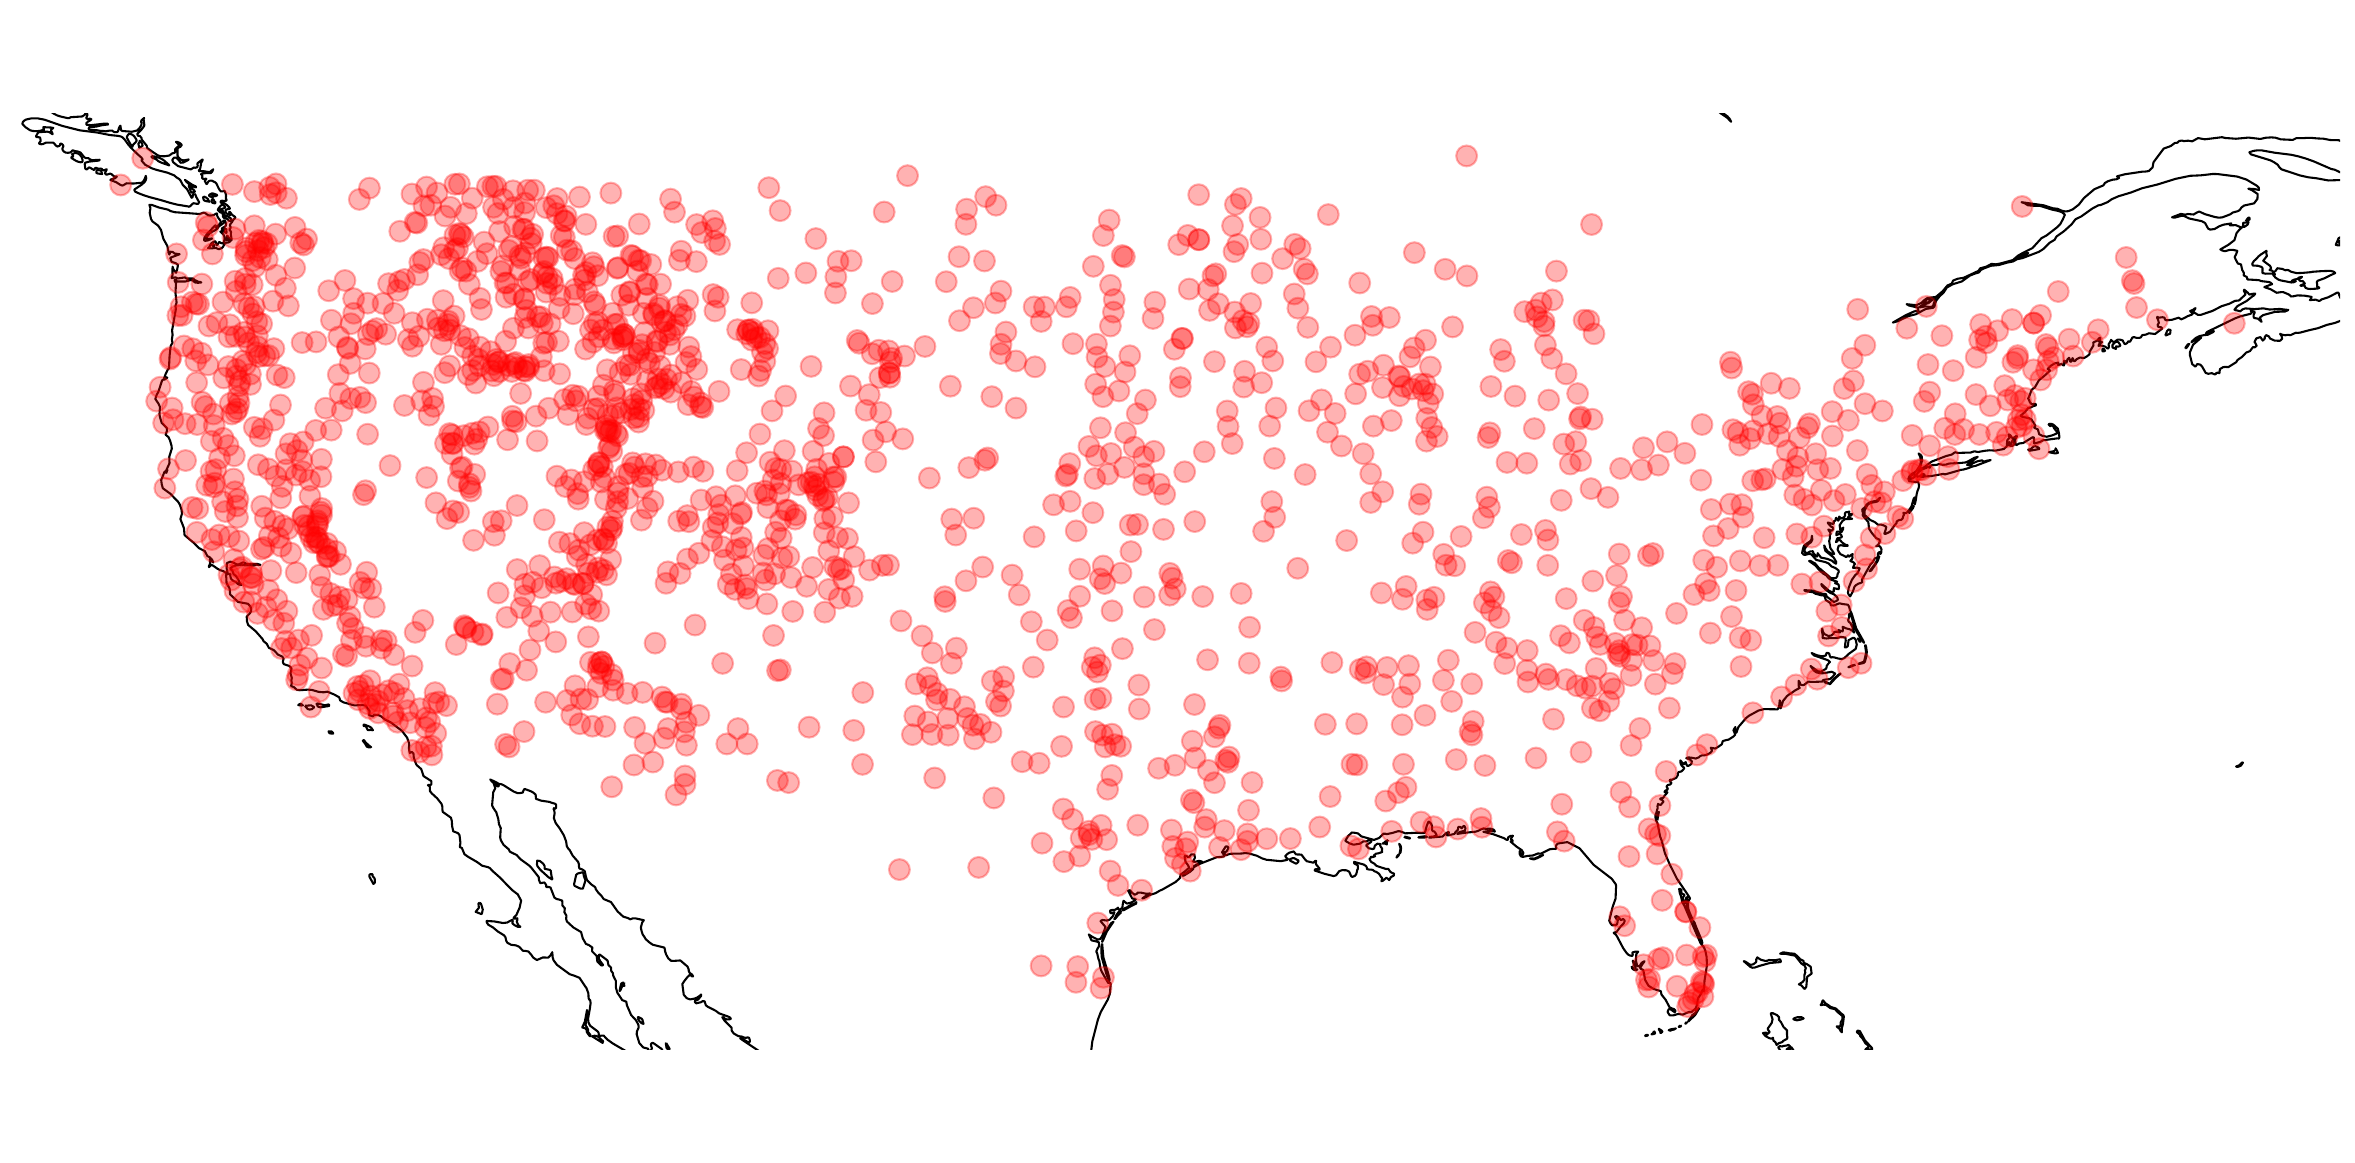}}
    \qquad
    \subfigure{\includegraphics[width=0.26\linewidth]{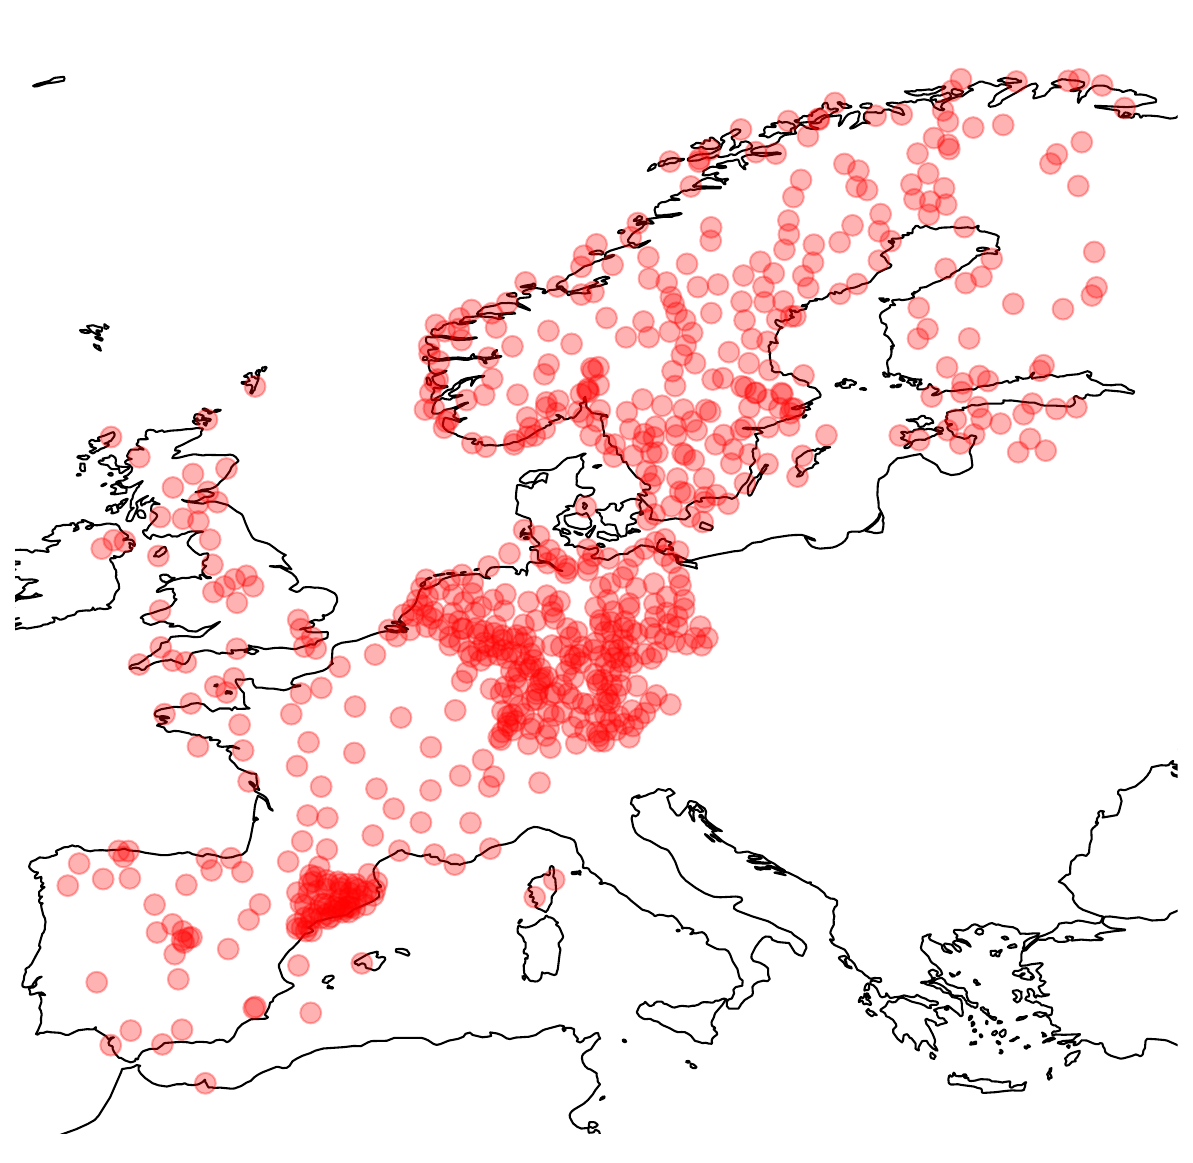}}
    \caption{(left) GHCN weather stations in the USA and (right) GHCN weather stations in Europe.}
    \label{fig:append-ghcn}
    % \vspace{-4mm}
\end{figure}

\begin{table*}[h]
% \vspace{-1em}
\centering
\small
\begin{tabular}{@{}ccccccc@{}}
\toprule
& GCN & GAT & GraphSAGE & GN & PA-DGN & {\ours} \\ \midrule
\# of parameters & 10,801 & 11,203 & 21,401 & 20,385 & 33,795 & 33,795 \\ \bottomrule
\end{tabular}
\caption{The number of learnable parameters for baselines and {\ours}}
\label{tab:append-num-params}
\end{table*}

\begin{table*}[]
    \centering
    \begin{tabular}{cccc}
    \toprule
          & $(N,F)=(700,1.5)$ & $(N,F)=(1700,2)$ & $(N,F)=(128,7)$ \\ \midrule
        5-shot & \textbf{0.781$\pm$0.019} & 0.981$\pm$0.131 & 1.007$\pm$0.096 \\ 
        10-shot & \textbf{0.773$\pm$0.014} & 0.951$\pm$0.151 & 0.932$\pm$0.058 \\ \bottomrule 
    \end{tabular}
    \caption{Regression error (MAE, $10^{-3}$) of different topology for synthetic dynamics (Europe)}
    \label{tab:append-ablation}
\end{table*}

\section{Task 2: Graph Signal Regression} \label{sec:append-task2}

\subsection{Meta-train}
\textbf{Data}: For the graph signal regression task, we generate synthetic dynamics for meta-train tasks and the synthetic data is adapted to a target dataset.
Before setting the topological configuration for the synthetic dynamics, we first examine the target dataset to understand its topological properties.
Based on the number of stations and the scale of records, we tune the topological configuration for the synthetic dataset.
We use $(N,F)=(1700,2)$ for the USA records and $(N,F)=(700,1.5)$ for Europe records, respectively, and 100 different initial values are generated to define different tasks.
Fig.~\ref{fig:append-ghcn} visualizes how the regional stations are distributed and Fig.~\ref{fig:append-ghcn-syn} demonstrates how the spatial distribution of synthetic nodes and scales of synthetic values are adapted to the corresponding target dynamics.

\subsection{Meta-test}
\textbf{Data}: The GHCN-Daily summaries from land surface stations across the globe provide daily climate records from numerous sources\footnote{Global Historical Climatology Network (GHCN) provided by National Oceanic and Atmospheric Administration (NOAA). https://www.ncdc.noaa.gov/ghcn-daily-description}. 
As the records from 100,000 stations in 180 countries and territories, the distribution of the weather stations is spatially non-uniform.
We sample sensors from two different regions (1) the USA and (2) Europe and construct a graph structure from the regional stations based on $k$-NN algorithm ($k=4$) as described in~\cite{defferrard2019deepsphere}.
There are 1,705 and 703 fully functioning sensors in the USA and Europe, respectively.
We use 2010 year records and first few daily records for few-shot training (5 and 10) and next 100/150 days for validation and test.
Note that the number of learnable parameters is significantly reduced compared to those of the previous task to minimize overfitting as well as be comparable to other variants of graph neural networks.

\subsection{Experimental Details}

\subsubsection{Baselines}
Since the input length of the regression task is fixed (length=5), we can consider many variants of graph neural networks for the task.
We concatenate the 5-step signals and feed it into Graph convolutional networks (\textbf{GCN})~\cite{kipf2016semi}, Graph attention networks (\textbf{GAT})~\cite{velickovic2018graph}, \textbf{GraphSAGE}~\cite{hamilton2017inductive}, and Graph networks (\textbf{GN})~\cite{sanchez2018graph} to predict next signals across all nodes.
For the baselines, we commonly consider 3-hop neighbors of $i$-th node to predict of the $i$-th node and the number of learnable parameters is similar to provide similar expressive power.

% \subsubsection{Ours}

% \textbf{PiMetaL}: Meta-train the spatial derivative modules (SDM) with our proposed Alg. 3 on the meta-train tasks generated in~\ref{ap:meta-train}.
% Then for each meta-test task, initialize one time derivative module (TDM) randomly and output of SDM is fed into the TDM to train it on the single task.
% The architecture for SDM and TDM are identical for the spatial derivative layer and the recurrent graph network in PA-DGN, respectively.

\section{Sensitivity Analysis of Synthetic Dynamics}
It is important to study how much the model's performance is dependent on synthetic topology.
In this section, we conduct an ablation study to see whether different choices of the synthetic topology affects the performance significantly or not.
According to Table~\ref{tab:ghcn-exp}, the regression error is fairly converged from a few samples for the Europe records. 
Thus, we apply different synthetic topology for the data to see if the saturated regression error is significantly changed.
For this ablation study, we reuse the synthetic dynamics adapted for the USA records and generate one more synthetic dynamics for spatially low-resolution cases.

Table~\ref{tab:append-ablation} shows that the regression performance across different topology is stable regardless of the number of shots, however, it is significantly degraded when we change the synthetic topology from the adapted one ($(N,F)=(700,1.5)$) for meta-training.
When we increase the spatial resolution ($N=700\rightarrow1700$), the meta-initialized spatial modules are adapted to learn spatial derivatives defined on spatially higher resolution. 
In such case, SDM likely assigns high weights to directly adjacent nodes as well as farther nodes (e.g., 3-hop nodes) as all neighbor nodes are strongly associated with exact spatial derivatives.
On the other hand, if SDM is meta-initialized from a lower resolution ($N=700\rightarrow128$), further nodes are too much underestimated.
Thus, it is important to construct proper topology for transferring the PDE-independent representations from synthetic dynamics to target dynamics.
